# Supplementary material for: Predicting and controlling nonlinear neuro-mechanical locomotion dynamics
Source: arXiv:2605.03362 source file (2026-05-05)
Supplement: Supplementary file 1 [file _combined_supp.tex]

\input{Main_format/packages}

\setcounter{figure}{0}
\setcounter{equation}{0}
\setcounter{table}{0}
\setcounter{section}{0}

% bibliography
\bibliographystyle{naturemag}

\hypersetup{hidelinks}

% paragraph
\linespread{1.3}

%Figure caption
\DeclareCaptionJustification{justified}{\justifying}

% geometry
\usepackage[a4paper, total={7in, 10in}]{geometry}

\input{Main_format/symbols}
